# Supplementary material for: PDE constrained shape optimisation with first-order and Newton-type methods in the $W^{1,\infty}$ topology
Source: arXiv:2301.08690 source file (2023-12-21)
Supplement: Supplementary file 1 [file appendix.tex]

\begin{lemma}\label{lem:BiHarmonicShapeDerivative}
Let $\mathcal J$ be given by
\begin{equation}
    \mathcal J(\Omega) = \int_\Omega j(\cdot,y_1)
\end{equation}
where $j\colon D \times \R \to \R$ is given and $y \in \left( H^1_0(\Omega) \right)^2$ satisfies
\begin{align}
    \int_\Omega \nabla y_2 \cdot \nabla \eta_1 &= \int_\Omega F \eta_1 \quad \forall \eta_1 \in H^1_0(\Omega),
    \\
    \int_\Omega \nabla y_1 \cdot \nabla \eta_2 &= \int_\Omega v \eta_2  \quad \forall \eta_2 \in H^1_0(\Omega)
\end{align}
for some given $F \in L^2_{loc}(\R^d)$.
Let $p \in \left( H^1_0(\Omega) \right)^2$ satisfy
\begin{align}
    \int_\Omega \nabla p_2 \cdot \nabla \eta_1 &= -\int_\Omega j_y(\cdot,y_1)[\eta_1] \quad \forall \eta_1 \in H^1_0(\Omega),
    \label{eq:appendixAdjointBiharmonic1}
    \\
    \int_\Omega \nabla p_1 \cdot \nabla \eta_2 &= \int_\Omega p_2 \eta_2  \quad \forall \eta_2 \in H^1_0(\Omega).
    \label{eq:appendixAdjointBiharmonic2}
\end{align}
The shape derivative $\mathcal{J}'(\Omega)[V]$ is given by
\begin{equation}
    \begin{split}
        \mathcal{J}'(\Omega)[V]
        =&
        \int_\Omega j(\cdot,y_1) \Div V + j_u(\cdot,y_1)[V]
        +
        \A V \nabla y_1 \cdot \nabla p_2
        \\
        &-
        y_2 p_2 \Div V + \A V \nabla y_2 \cdot \nabla p_1
        - \Div (V F) p_1
    \end{split}
\end{equation}
\end{lemma}
\begin{proof}
For convenience, let us write $v = y_2$ and $y = y_1$.
Letting $\Phi_t = \id + tV$, one has that $\mathcal{J}(\Omega_t) = \int_\Omega j(\Phi_t, y_t \circ \Phi_t) \det(D\Phi_t)$.
Taking its derivative gives
\begin{equation}
    \mathcal{J}'(\Omega)[V] = \int_\Omega j(\cdot,y) \Div V + j_u(\cdot,y)[V] + j_y(\cdot, y)\left[ \left.\frac{\dee}{\dee t}\right|_{t=0} (y_t \circ \Phi_t)\right].
\end{equation}
Let us write $Y:=\left.\frac{\dee}{\dee t}\right|_{t=0} (y_t \circ \Phi_t)$ and $w := \left.\frac{\dee}{\dee t}\right|_{t=0} (v_t \circ \Phi_t)$ which satisfy
\begin{align}
    \int_\Omega \nabla w \cdot \nabla \eta + \A V \nabla v \cdot \nabla \eta &= \int_\Omega V \cdot \nabla F \eta + \Div V F \eta \quad \forall \eta \in H^1_0(\Omega),
    \label{eq:appendixDerivativeBiharmonic1}
    \\
    \int_\Omega \nabla Y \cdot \nabla \xi + \A V \nabla y \cdot \nabla \xi &= \int_\Omega w \xi + \Div V v \xi \quad \forall \xi \in H^1_0(\Omega).
    \label{eq:appendixDerivativeBiharmonic2}
\end{align}
Taking $\eta = Y$ in \eqref{eq:appendixAdjointBiharmonic1}, $\xi = p$ in \eqref{eq:appendixDerivativeBiharmonic2}, $\xi = w$ in \eqref{eq:appendixAdjointBiharmonic2} and $\eta = q$ in \eqref{eq:appendixDerivativeBiharmonic1}, one sees that
\begin{align}
    \int_\Omega j_y(\cdot,y)[Y]
    =&
    -\int_\Omega \nabla Y \cdot \nabla q
    =
    \int_\Omega \A V \nabla y \cdot \nabla q - wq - \Div V v q,
    \\
    -\int_\Omega w q
    =&
    - \int_\Omega \nabla p \cdot \nabla q
    =
    \int_\Omega \A V \nabla v \cdot \nabla p - V\cdot \nabla F  p - \Div V F p,
\end{align}
from which it holds
\begin{align}
    \int_\Omega j_y(\cdot,y)[Y]
    =&
    \int_\Omega \A V \nabla y \cdot \nabla q - \Div V v q
    +
    \A V \nabla v \cdot \nabla p - \Div ( V\nabla F) p
\end{align}
and the result follows.
\end{proof}
